# Supplementary material for: Efficient and Scalable Structure Learning for Bayesian Networks: Algorithms and Applications
Source: arXiv:2012.03540 source file (2020-12-07)
Supplement: Supplementary file 1 [file appendix.tex]

\newpage

\section*{Supplementary Materials}

In this supplementary document, we provide the detailed proofs of all lemmas in this paper.  

\setcounter{lemma}{0}

\begin{lemma}
For any non-negative matrix $\S$, $k \geq 0$ and $0 \leq \alpha \leq 1$, the spectral radius $\delta$ of matrix $\S$ is no larger than $\uppdelta^{(k)}$.
\end{lemma}

\proof
Let $\delta^{(k)}$ denote the exact spectral radius of matrix $\S^{(k)}$. We first prove that $\delta^{(k)} \leq \uppdelta^{(k)}$. According to the upper bound on the spectral radius of matrices in~\cite{Surhone2011Spectral}, since $\S^{(k)}$ is a non-negative matrix, we have 
\begin{equation*}
\begin{split}
\delta^{(k)} & \leq \max_{1 \leq i \leq d} { \left(r(\S^{(k)})[i] \right)}^{\alpha} { \left(c(\S^{(k)})[i] \right )}^{1 - \alpha} \\
& \leq \sum_{i = 1}^{d}  { \left(r(\S^{(k)})[i] \right)}^{\alpha} { \left(c(\S^{(k)})[i] \right )}^{1 - \alpha}  = \sum_{i = 1}^{d} b^{(k)}[i] = \uppdelta^{(k)}.
\end{split}
\end{equation*}
Then by Eq.~\eqref{eq: uppdelta}, for any $k \geq 0$, $\S^{(k + 1)}$ is a matrix similar to $\S^{(k)}$, so they have the same spectral radius. Therefore, we have $\delta = \delta^{(k)} = \delta^{(0)} \leq \uppdelta^{(k)}$.
\proofend

\begin{lemma}
	\label{lem: consisybound}
	For any non-negative matrix $\S$, $k \geq 0$ and any value $0 < \epsilon, \alpha < 1$, 
	if the upper bound $\uppdelta^{(k)} \leq \ln(\frac{\epsilon}{d} + 1)$, then
	$h(\S) \leq \epsilon$ holds; if the upper bound $\uppdelta^{(k)} \leq \frac{1}{\alpha} \log_{d} \frac{\epsilon}{d^{2}}$, then $g(\S) \leq \epsilon$ holds.
\end{lemma}

\proof
By Eq.~\eqref{eq: wdag}, we have
\begin{equation*}
h(\S) = \sum_{t = 1}^{\infty} \frac{\text{Tr}(\S^{t})}{t!} 
= \sum_{t = 1}^{\infty} \left(\frac{1}{t!} \sum_{i = 1}^{d}  \delta_{i}^{t} \right)
\leq \sum_{t = 1}^{\infty}  \frac{d {\uppdelta^{(k)}}^{t}}{t!} = d(e^{\uppdelta^{(k)}} - 1).
\end{equation*}
Therefore, if we have $\uppdelta^{(k)} \leq \ln(\frac{\epsilon}{d} + 1)$, we must have $h(\S) \leq \epsilon$.

By Eq.~\eqref{eq: wdagnew}, we have
\begin{equation*}
\begin{split}
g(\S) & =  \sum_{t = 1}^{d} {d \choose t} \alpha^{t} \text{Tr}(\S^{t}) \\
& = \sum_{t = 1}^{d} {d \choose t} \alpha^{t} \sum_{i = 1}^{d}  \delta_{i}^{t}
\leq d \sum_{t = 1}^{d} {d \choose t} \alpha^{t} {\uppdelta^{(k)}}^{t}
= d {(1 + \alpha \uppdelta^{(k)})}^{d}.
\end{split}
\end{equation*}
Therefore, if we have $\uppdelta^{(k)} \leq \frac{1}{\alpha} \log_{d} \frac{\epsilon}{d^{2}}$, we must have $g(\S) \leq \epsilon$.
\proofend

\begin{lemma}
For any non-negative matrix $\S$, $k \geq 0$ and $0 \leq \alpha \leq 1$, we always have
$\grd_{\S^{(k)}} \uppdelta^{(k)}  = \grd_{\S^{(k)}} b^{(k)}  = x^{(k)} \circ \mathbf{1} + {(y^{(k)})}^{T} \circ \mathbf{1}$, 
where $x^{(k)} = \alpha { \left(\frac{{c (\S^{(k)})}}{r(\S^{(k)})} \right)}^{1 - \alpha} $, $y^{(k)} = (1 - \alpha) { \left(\frac{{r(\S^{(k)})}}{{{c(\S^{(k)})}}} \right)}^{\alpha}$, and $\mathbf{1} \in \mathbb{R}^{d \times d}$ is a matrix with all elements equal to $1$.
\end{lemma}

\proof
Since $\uppdelta^{(k)} = \sum_{i = 1}^{d} b^{(k)}[i]$, we have
\begin{equation*}
\grd_{\S^{(k)}} \uppdelta^{(k)} = \grd_{b^{(k)}} \uppdelta^{(k)} \circ \grd_{\S^{(k)}} b^{(k)} = \mathbf{1} \circ \grd_{\S^{(k)}} b^{(k)} = \grd_{\S^{(k)}} b^{(k)}.
\end{equation*}
Then by Eq.~\eqref{eq: uppdelta} between $\S^{(k)}$ and $b^{(k)}$, we have
\begin{equation*}
\begin{split} 
\grd_{\S^{(k)}} \uppdelta^{(k)} & = \grd_{\S^{(k)}} \left( {(r(\S^{(k)}))}^{\alpha} \circ {(c(\S^{(k)}))}^{1 - \alpha} \right) \\
& = {({r(\S^{(k)})^{T})}}^{\alpha} \circ \grd_{\S^{(k)}} \left({(c(\S^{(k)}))}^{1 - \alpha} \right) \\
& + {{{(c(\S^{(k)}))}}^{1 - \alpha}} \circ \grd_{\S^{(k)}} \left( {(r(\S^{(k)}))}^{\alpha}  \right) \\
& = (1 - \alpha) {({r(\S^{(k)})}^{T})}^{\alpha} \circ {({c(\S^{(k)})}^{T})}^{-\alpha} \circ \mathbf{1} \\
& + \alpha {(c(\S^{(k)}))}^{1 - \alpha} \circ {(r(\S^{(k)}))}^{\alpha - 1} \circ \mathbf{1} \\
& = x^{(k)} \circ \mathbf{1} +  {(y^{(k)})}^{T} \circ \mathbf{1}.
\end{split}
\end{equation*}
Thus, the lemma holds.
\proofend

\begin{lemma}
	For any non-negative matrix $\S$, $k \geq 1$ and $0 \leq \alpha \leq 1$, 
	given any $1 \leq j \leq k$, suppose that we already obtained $\grd_{\S^{(j)}} \uppdelta^{(k)}$,  we denote
	\begin{equation*}
	\begin{split}
	z^{(j - 1)} & = - \frac{r(\grd_{\S^{(j)}} \uppdelta^{(k)} \circ \S^{(j-1)} \circ {(b^{(j-1)})}^{T} )}{{(b^{(j - 1)})}^{2}} \\
	& + c( {(b^{(j - 1)})}^{-1} \circ \grd_{\S^{(j)}} \uppdelta^{(k)} \circ \S^{(j - 1)}).
	\end{split}
	\end{equation*}
	Then, we have
	
	\begin{equation*}
	\begin{split}
	\grd_{\S^{(j - 1)}} \uppdelta^{(k)}  & =  {(b^{(j - 1)})}^{-1} \circ \grd_{\S^{(j)}} \uppdelta^{(k)} \circ 
	{(b^{(j - 1)})}^{T} \\
	& + x^{(j - 1)} \circ z^{(j - 1)} \circ \mathbf{1} + {(y^{(j - 1)})}^{T} \circ {(z^{(j - 1)})}^{T} \circ \mathbf{1}
	\end{split}
	\end{equation*}
	where $x^{(j - 1)}$ and $y^{(j - 1)}$ have the same meaning as in Lemma~\ref{lem: grdD2S}.
\end{lemma}

\proof
Suppose that we have already obtained $\grd_{\S^{(j)}} \uppdelta^{(k)}$, we then show how to obtain 
$\grd_{\S^{(j - 1)}} \uppdelta^{(k)}$. Let $\U^{(j)}$ denote $\S^{(j)} \circ {(b^{(j)})}^{T}$. 
By Eq.~\eqref{eq: mulskd}, we have $\S^{(j)} = \U^{(j - 1)} \circ {(b^{(j - 1)})}^{-1}$. Obviously, we have
\begin{equation*}
\grd_{\U^{(j - 1)}} \uppdelta^{(k)} = \grd_{\S^{(j)}} \uppdelta^{(k)} \circ {(b^{(j)})}^{T}, 
\end{equation*}
and 
\begin{equation*}
\grd_{{(b^{(j - 1)})}^{-1}} \uppdelta^{(k)} = r(\grd_{\S^{(j)}} \uppdelta^{(k)} \circ (\U^{(j - 1)})).
\end{equation*}
Since $\grd_{b^{(j - 1)}} {(b^{(j - 1)})}^{-1} = - {(b^{(j - 1)})}^{-2}$, we have
\begin{equation*}
\begin{split}
\grd_{{(b^{(j - 1)})}} \uppdelta^{(k)} & = \grd_{{(b^{(j - 1)})}^{-1}} \uppdelta^{(k)} \circ \grd_{b^{(j - 1)}} {(b^{(j - 1)})}^{-1} \\
& + c(\S^{(j - 1)} \circ \grd_{\U^{(j - 1)}} \uppdelta^{(k)}) \\
& = - \frac{r(\grd_{\S^{(j)}} \uppdelta^{(k)} \circ \S^{(j-1)} \circ {(b^{(j-1)})}^{T} )}{{(b^{(j - 1)})}^{2}} \\
& + c( {(b^{(j - 1)})}^{-1} \circ \grd_{\S^{(j)}} \uppdelta^{(k)} \circ \S^{(j - 1)}) \\
& = z^{(j - 1)}.
\end{split}
\end{equation*}
Then, similar to the proof process of Lemma~\ref{lem: grdD2S}, we have 
\begin{equation*}
\begin{split}
\grd_{\S^{(j - 1)}} \uppdelta^{(k)}  & =  {(b^{(j - 1)})}^{-1} \circ \grd_{\S^{(j)}} \uppdelta^{(k)} \circ 
{(b^{(j - 1)})}^{T} \\
& + x^{(j - 1)} \circ z^{(j - 1)} \circ \mathbf{1} + {(y^{(j - 1)})}^{T} \circ {(z^{(j - 1)})}^{T} \circ \mathbf{1}
\end{split}
\end{equation*}
Thus, the lemma holds.
\proofend

\begin{lemma}
For any matrix $\W$, $k \geq 1$ and $0 \leq \alpha \leq 1$, let $\M \in \mathbb{R}^{d \times d}$ be such that $\M[i, j] = 1$ when $\W[i, j] \neq 0$ and $\M[i, j] = 0$ otherwise. Let
$\grd'_{\S^{(k)}} \uppdelta^{(k)}  = x^{(k)} \circ \M  + {(y^{(k)})}^{T} \circ \M$. For all $1 \leq j \leq k - 1$, let
	\begin{equation*}
	\begin{split}
	\grd'_{\S^{(j - 1)}} \uppdelta^{(k)}  & =  {(b^{(j - 1)})}^{-1} \circ \grd'_{\S^{(j)}} \uppdelta^{(k)} \circ 
	{(b^{(j - 1)})}^{T} \\
	& + {x}^{(j - 1)} \circ z^{(j - 1)} \circ \mathbf{M} + {(y^{(j - 1)})}^{T} \circ {(z^{(j - 1)})}^{T} \circ \mathbf{M}
	\end{split}
	\end{equation*}
	where $x^{(j - 1)}$ and $y^{(j - 1)}$ are defined in Lemma~\ref{lem: grdD2S},
	and $z^{(j - 1)}$ is defined in Eq.~\eqref{eq: grdzj}.
	Then, we always have
	\begin{equation*}
	\grd_{\W} \uppdelta^{(k)} = 2 \grd'_{\S} \uppdelta^{(k)} \circ \W.
	\end{equation*}
\end{lemma}

\proof
Since all vectors $x^{(j - 1)}$ and $y^{(j - 1)}$ are computed by the matrices $\S^{(j - 1)}$, their values always keep same for each $j$ no matter we use the matrix $\M$ or not. Meanwhile, by 
Eq.~\eqref{eq: mulskd} and the definition of matrix $\M$, obviously we have $\S^{(j)} \circ \M = \S^{(j)}$ for all $j \geq 0$. Therefore, replacing $\grd_{\S^{(j)}} \uppdelta^{(k)}$ to $\grd'_{\S^{(j)}} \uppdelta^{(k)}$ would not change the value of vector $z^{(j - 1)}$ for all $j \geq 1$. That means only the elements in $\grd_{\S^{(j)}} \uppdelta^{(k)}$ which are in a non-zero position in $\M$ contributes to computing $z^{(j - 1)}$. As a result, we can safely remove all other elements in $\grd_{\S^{(j)}} \uppdelta^{(k)}$ to obtain $\grd'_{\S^{(j)}} \uppdelta^{(k)}$. Finally, we obviously have 
$\grd_{\W} \uppdelta^{(k)} =  2 \grd_{\S} \uppdelta^{(k)} \circ \W = 2 \grd'_{\S} \uppdelta^{(k)} \circ \W$.
\proofend

\begin{lemma}
If $f_{i}(X)$ is defined as in Eq.~\eqref{eq: fXNN}, let $ r_{ij} = \prod_{k = 1}^{K} {\| \H^{(k)}_{i} [ : j] \|_{2}}$, 
	where $\H^{(k)}_{i} [ : j]$ is the $j$-th column of the matrix $\H^{(k)}_{i}$. 
	Then, if $r_{ij} = 0$ we must have $f_{i}(X)$ does not depend on $X_j$.
\end{lemma}

\proof
Obviously, $r_{ij} = 0$ indicates that $\H^{(k)}_{i} [t : j] = 0$ for all $1 \leq k \leq K$ and $1 \leq t \leq d$. By Eq.~\eqref{eq: fXNN}, we always have 
\begin{equation*}
\left( \H^{(k)}_{i} \dots \phi^{(2)}_{i} (\H^{(2)}_{i} \phi^{(1)}_{i} (\H^{(1)}_{i} X)) \right)[j] = 0
\end{equation*}
for all $1 \leq k \leq K$. Therefore, $f_{i}(X) [j] = \phi^{(K)}_{i} (0)$ is a fixed value and does not depend on $X_j$. 
\proofend
